# Supplementary material for: Smoothed Online Learning for Prediction in Piecewise Affine Systems
Source: arXiv:2301.11187 source file (2024-03-19)
Supplement: Supplementary file 1 [file related_work.tex]

\subsection{Related Work}
\paragraph{System Identification. } System-identification refers to estimating the governing equations of a dynamical system. The special case of linear dynamical systems is classical \citep{ljung1999system,ljung1992asymptotic,deistler1995consistency}, and more recent work has provided finite-sample statistical analyses in many regimes of interest \citep{simchowitz2018learning,dean2017sample,oymak2019non,tsiamis2019finite,tsiamis2022statistical}. Estimation for non-linear systems has proven challenging, and has been studied most in the setting where the dynamics involve a known and smooth nonlinearity \citep{mania2020active,sattar2020non,foster2020learning}, or where only the observation model is nonlinear \citep{dean2021certainty,mhammedi2020learning}. \cite{sattar2021identification} study \emph{Markov jump systems}, where the system dynamics alternate between one of a finite number of linear systems (``modes''), with switches between modes governed by a Markov chain.  PWA systems are thus an attractive intermediate step between the simple linear setting and the intractable general case.  To our knowledge, ours is the first work to tackle piecewise affine dynamics in full generality, where the system mode is determined by the system state.

% \paragraph{Heuristics for PWA System Identification.} 
\iftoggle{icml}{}{\begin{sloppypar}}Despite its worst-case computational intractability \citep{amaldi2002min}, there is a rich literature of heuristic algorithms for computing the best-fit PWA system to data; see the surveys \cite{garulli2012survey} and \cite{paoletti2007identification}, which compare various approaches, notably the clustering method due to \cite{ferrari2003clustering}. These references focus strictly on the \emph{algorithmic} facets of computing a best-fit given an existing data set. We instead abstract the computation of a best-fit into an ERM oracle in order to focus on the \emph{statistical} considerations. 
\iftoggle{icml}{}{\end{sloppypar}}

\paragraph{Online Learning and Smoothing. }  The study of online learning is now classical, with a small sample of early works including \citet{littlestone1988learning,freund1999large,freund1999adaptive}.  More recently, a general theory of online learning matching that which we have in the statistical learning setting was built up in \citet{rakhlin2011online,rakhlin2013online,rakhlin2015sequential,block2021majorizing}, with \citet{rakhlin2014online} characterizing the minimax regret of online regression.  Due to the robustness and generality of this adversarial model, many problems that are trivial to learn in the statistical setting become impossible in the adversarial regime.  Thus, some work \citep{rakhlin2011online,haghtalab2021smoothed,haghtalab2022oracle,block2022smoothed,block2023sample} has sought to constrain the adversary to be \emph{smooth}, in the sense that the adversary is unable to concentrate its actions on worst-case points.  In addition, \citet{block2022efficient}, which introduces the notion of directional smoothness to control the regret in a realizable, online classification problem; realizability, here, means that there is no process noise in the sense that there exists some piecewise affine function that perfectly predicts all targets given the covariates.  We also note that the algorithm in that paper is highly tailored to this realizable setting and thus is not at all robust to the noise considered in the present paper.  Of particular note is the concurrent work of \citet{block2023oracle}, which solves a similar problem with a stronger oracle.  Note that in that paper, the oracle assumption is strong enough to break the lower bound of \citet{hazan2016computational}, while in this work we use the much weaker oracle assumption found in \citet{hazan2016computational,haghtalab2022oracle,block2022smoothed}.  This distinction is important because even in the standard (fully adversarial) online learning setting, there is a computational separation between these two oracle models in general, as per \citet{agarwal2019learning}; thus the fact that this separation does not apply to PWA systems given smoothness may be of independent interest.

\paragraph{Online Learning for Control.} In addition to the recent advances in finite-sample system identification, a vast body of work has studied control tasks from the perspective of regret \citep{abbasi2011regret,agarwal2019online,simchowitz2020improper,simchowitz2020naive,cohen2018online}. While we do not consider a control objective in this work, we share with these works the performance metric of regret. Our work is more similar in spirit to online prediction in control settings \citep{hazan2017learning,tsiamis2020sample}, in that we also consider the task of next-step predictions under a system subject to control inputs. 

\paragraph{Smoothing in RL and Control.} One interpretation of the smooth online learning setting is that well-conditioned random noise is injected into the adversary's decisions.  It is well known that such noise injection can be viewed as a form of regularization \citep{duchi2012randomized}, and recent recent work in the robotics literature has shown that randomized smoothing improves the landscape in various robotic planning and control tasks  \citep{suh2022differentiable,suh2022bundled,lidec2022leveraging,pang2022global}. More broadly, randomization has been popular for computation of zeroth-order estimates of gradients, notably via the acclaimed policy-gradient computation \cite{williams1992simple}.
